# Supplementary material for: The More, the Better? A Study on Collaborative Machine Learning for DGA Detection
Source: arXiv:2109.11830 source file (2021-09-24)
Supplement: Supplementary file 1 [file appendix.tex]

% !TEX root = ../paper.tex
\section{Appendix}
\label{sec:appendix}
